# Supplementary material for: Controlled confinement of half-metallic two-dimensional electron gas in BaTiO3/Ba2FeReO6/BaTiO3 heterostructures: A first-principles study
Source: arXiv:1510.06805 source file (2015-10-23)
Supplement: Supplementary file 1 [file supplementary1.pdf]

# Supplemental Material
# Controlled Confinement of Half-metallic 2D Electron Gas in $BaTiO_3/Ba_2FeReO_6/BaTiO_3$ Heterostructures: A First-principles Study

Santu Baidya,[1] Umesh V Waghmare,[1] Arun Paramekanti,[2] and Tanusri Saha-Dasgupta[3]

[1]*Jawaharlal Nehru Centre for Advanced Scientific Research, Jakkur, Bangalore 560064, India*
[2]*Department of Physics, University of Toronto, Toronto, Ontario, Canada M5S 1A7*
[3]*S.N. Bose National Centre for Basic Sciences, Kolkata 700098, India*

## A. COMPUTATIONAL DETAILS OF DFT CALCULATIONS

In order to study the electronic structure of bulk BFRO as well as the heterostructures, we have carried out first principles DFT calculations with Perdew-Burke-Ernzerhof formulation of generalized gradient approximation (GGA).[1] We have used projector augmented-wave (PAW) potential[2, 3] as implemented in the Vienna *ab initio* simulation package (VASP) [4, 5]. Plane wave calculations are performed for optimization of the structure as well as for the calculation of electronic and magnetic properties. The energy cutoff for the plane wave expansion was chosen to be 700 eV. For structural optimization of heterostructure $13 \times 13 \times 2$ Monkhorst-Pack $k$-point mesh was used to have a force convergence of 0.01eV/Å. For self-consistent field calculation $13 \times 13 \times 2$ Monkhorst-Pack $k$-point mesh was used to have a good convergence for heterostructures while for bulk $Ba_2FeReO_6$ $8 \times 8 \times 8$ Monkhorst-Pack $k$-point mesh was used. The effect of spin-orbit coupling (SOC) has been included in the calculations as second variational form to the original Hamiltonian. The radii chosen in the plane wave basis set to calculate the partial density of states as well as site projected magnetic moments were 1.98 Å for Ba, 1.32 Å for Ti, 1.43 Å for Re, 1.30 Å for Fe and 0.9 Å for O atom.

The onsite energies of the low-energy tight-binding model for the Re $t_{2g}$ states and Fe $t_{2g}$ states are obtained from the muffin-tin orbital (MTO) based $N^{th}$ order MTO[6] (NMTO) method as implemented in Stuttgart code. Starting from a full DFT calculation, NMTO-downfolding calculation derives a few-orbital Hamiltonian, by integrating out degrees which are not of interest. It does so by defining energy-selected, effective orbitals which serve as Wannier-like orbitals defining the few-orbital Hamiltonian in the downfolded representation. To calculate the energy level positions of Fe $t_{2g}$'s and Re $t_{2g}$'s employing NMTO downfolding, we first downfold O $p$, Ba as well as Fe and Re $e_g$ degrees of freedom. This gives the energy level positions of Fe $t_{2g}$ and Re $t_{2g}$ states, in absence of hybridization between the two. We subsequently carry out massive downfolding, keeping only the Re $t_{2g}$ degrees of freedom active and downfolding everything else including Fe $t_{2g}$ degrees of freedom. This defines the renormalized Re $t_{2g}$ states taking into account hybridization effect between Fe $t_{2g}$ and Re $t_{2g}$ states. The NMTO method, for which the selfconsistent version is yet to be available, relies on the selfconsistent potentials borrowed from the linear MTO (LMTO)[7] calculations. The consistency of results between the plane-wave and muffin-tin orbital calculations has been cross-checked.

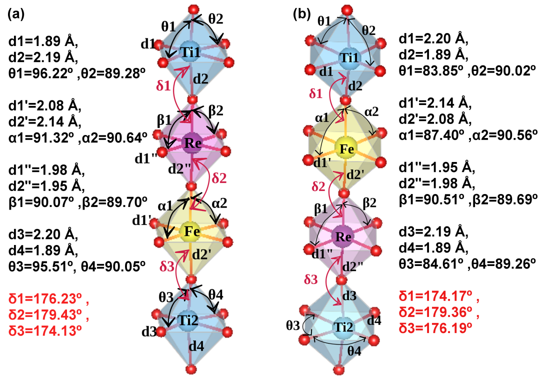


FIG. 1: The bond lengths and bond angles in the optimized heterostructure FE-BTO/BFRO/FE-BTO with two different initial structures.

## B. CALCULATIONS CONSIDERING THE FE PHASE OF BTO

To check the effect of ferroelectric highly polar structure of BTO(111) surfaces on the crystal structure of the heterostructure as well as on the electronic structure, we further carried out calculations considering the supercell of ferroelectric $BaTiO_3$ in rhombohedral perovskite structure[8, 9] oriented along [111] crystallographic direction, in which $Ba_2FeReO_6$ bilayer was sandwitched. The crystal structure of feroelectric(FE)-BTO/BFRO/FE-BTO heterostructure was then fully optimized. Furthermore to check the influence of the direction of the ferroelectric polarization in the heterostructure Fe and Re positions were exchanged and new FE-BTO/BRFO/FE-BTO structure was fully optimized again. No siginificant change in the crystal structure was observed between the two optimized structures, which to start with had two opposite direction of polarizations of BTO (refered as structure 1 and structure 2 in the following). The comparison of various bond angles and bond lengths between the two optimized structures corresponding to two initial structures with opposite directions of polarization in FE-BTO/BRFO/FE-BTO is shown in Fig 1. The comparison of calculated electronic structure confirmed that ferroelectricity of rhombohedral BTO does not induce any extra effect on the half-metallic,

confinded 2d elctron gas formed at BFRO bilayer. The calculated magnetic moments turn out to be rather similar (see Table I) confirming the little influence of ferroelectricity.

TABLE I: Calculated spin moments ($\mu_B$) corresponding to FE-BTO/BFRO/FE-BTO structure 1, FE-BTO/BRFO/FE-BTO/structure 2 and PE-BTO/BFRO/PE-BTO.

| | [structure 1] | [structure 2] | PE |
|---|---|---|---|
| Fe | -3.68 | -3.66 | -3.67 |
| Re | 0.82 | 0.87 | 0.84 |

## C. TIGHT BINDING MODEL FOR {111} BILAYER AND TOPOLOGICAL CHARACTER OF THE BILAYER BANDS

The three bands near the Fermi level have dominantly Re 5d-↑ character. They can be modelled using a tight-binding model for spin polarized electrons in $t_{2g}$ orbitals on the 2D triangular lattice formed by Re atoms on the $\{111\}$ face. This leads to a matrix Hamiltonian

$$H(\mathbf{k}) = \begin{pmatrix} \varepsilon^{yz}_{\mathbf{k}} & \beta+\gamma^z_{\mathbf{k}} & \beta^* + \gamma^y_{\mathbf{k}} \\ \beta^* + \gamma^z_{\mathbf{k}} & \varepsilon^{xz}_{\mathbf{k}} & \beta + \gamma^x_{\mathbf{k}} \\ \beta + \gamma^y_{\mathbf{k}} & \beta^* + \gamma^x_{\mathbf{k}} & \varepsilon^{xy}_{\mathbf{k}} \end{pmatrix} \quad (1)$$

where $\beta = -\frac{\Delta}{3} - i\frac{\lambda}{2\sqrt{3}}$, with $\Delta$ being the trigonal distortion ($\Delta > 0$ leads to compression along the trigonal axis), and $\lambda$ being the SOC coupling. The intra-orbital dispersions are

$$\varepsilon^{yz}_{\mathbf{k}} = -2t_{\|} \cos k_c - 2t_{\perp}(\cos k_a + \cos k_b) \quad (2)$$
$$\varepsilon^{xz}_{\mathbf{k}} = -2t_{\|} \cos k_b - 2t_{\perp}(\cos k_a + \cos k_c) \quad (3)$$
$$\varepsilon^{xy}_{\mathbf{k}} = -2t_{\|} \cos k_a - 2t_{\perp}(\cos k_b + \cos k_c), \quad (4)$$

and the inter-orbital dispersions are $\gamma^x_{\mathbf{k}} = -2t_m \cos k_c$, $\gamma^y_{\mathbf{k}} = -2t_m \cos k_b$, and $\gamma^z_{\mathbf{k}} = -2t_m \cos k_a$. Here we have defined $k_{a,b,c} = \mathbf{k}.\{\hat{a}, \hat{b}, \hat{c}\}$, with $\hat{a} = \hat{x}$, $\hat{b} = \hat{x}/2 + \hat{y}\sqrt{3}/2$, and $\hat{c} = \hat{b} - \hat{a}$, with distances being measured in units of the Re-Re distance. As shown in Fig. 2, a good fit to the *ab initio* band dispersion is obtained using the parameter set $t_{\|} = 200$meV, $t_{\perp} = -2$meV, $\Delta = 40$meV, $\lambda = 160$meV, and $t_m = 12$meV.

The Chern number of the $n^{th}$ band, or equivalently its TKNN index [10], is given by

$$C_n = \sum_{n' \neq n} \int \frac{d^2\mathbf{k}}{2\pi} \, \mathrm{Im} \frac{\langle n\mathbf{k}|v_x(\mathbf{k})|n'\mathbf{k}\rangle\langle n'\mathbf{k}|v_y(\mathbf{k})|n\mathbf{k}\rangle}{(E_n(\mathbf{k}) - E_{n'}(\mathbf{k}))^2} \quad (5)$$

where $v_i(\mathbf{k}) = \partial H(\mathbf{k})/\partial k_i$ is the velocity matrix (operator), $|n\mathbf{k}\rangle$ refers to the Bloch wavefunction of band-$n$ at momentum $\mathbf{k}$, and $E_n(\mathbf{k})$ is the corresponding band energy. Computing $C_n$ for the computed dispersion, we find that the three bands, in increasing order of energy at the $\Gamma$-point, have Chern numbers $-2, 2, 0$.

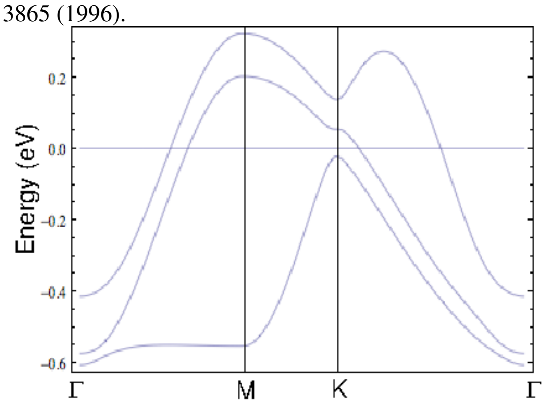


FIG. 2: Tight binding band dispersion for the $\{111\}$ bilayer, showing the three isolated bands which originate from Re $t_{2g}$ orbitals.

[1] J. P. Perdew, K. Burke, and M. Ernzerhof, Phys. Rev. Lett. **77**, 3865 (1996).
[2] P. E. Blöchl, Phys. Rev. B **50**, 17953 (1994).
[3] G. Kresse and D. Joubert, Phys. Rev. B **59**, 1758 (1999).
[4] G. Kresse and J. Hafner, Phys. Rev. B **47**, 558 (1993).
[5] G. Kresse and J. Furthmüller, Phys. Rev. B **54**,11169 (1996).
[6] O. K. Andersen and T. Saha-Dasgupta, Phys. Rev. B **62**, R16219 (2000).
[7] O. K. Andersen and O. Jepsen, Phys. Rev. Lett. **53**, 2571 (1984).
[8] A. W. Hewat, Ferroelectrics **6**, 215 (1974).
[9] G. H. Kwei, A. C. Lawson, S. J. L. Billinge and S.-W. Cheong, J . Phys. Chem. **97**, 2368 (1993).
[10] D. J. Thouless, M. Kohmoto, M. P. Nightingale, and M. den Nijs, Phys. Rev. Lett. **49**, 405 (1982).
